# Supplementary material for: Robust Consensus in Ranking Data Analysis: Definitions, Properties and Computational Issues
Source: arXiv:2303.12878 source file (2023-03-22)
Supplement: Supplementary file 1 [file X_appendix.tex]

\section{Distributionally Robust Optimization (DRO)}

Distributionally Robust Optimization (DRO) is a classical setting for incorporating risk-aversion, used in various statistical learning communities. In the context of ranking, this notion has not \intodo{Sure?} been defined and used yet. We propose to extend the DRO statistic to ranking data.

\begin{definition}\label{def:dro}
    {\sc{DRO Statistic}} Let $p\in\cM_+^1(\pS)$ and $d$ be a metric on $\pS$. The DRO statistic is defined by:
    \begin{align*}
        \sigma^{DRO}_{d, p} \in \argmin_{\sigma \in \pS} \max_{q | TV(p,q) \leq \varepsilon} \mathbb{E}_{\Sigma \sim q}(d(\sigma, \Sigma))\,.
    \end{align*}
\end{definition}

As the DRO statistic inherently optimize on the worst-case adversarial distribution for $p$ (which is reminiscent, but not necessarilly equivalent, of the inner term in the breakdown function definition), it makes a good robust statistic candidate. 

\paragraph{Bucket orders are solution for the DRO.} \cref{sec:setting} briefly mentioned the intuition that letting bucket orders be the output of statistics is a good approach to increase robustness. The DRO statistic motivates this remark because it can be shown that for some distributions $p\in\cM_+^1(\pS)$, whe have $\pi^{DRO}_{p,H} \in \Pi_n \setminus \frak{S}_n$, meaning that bucket orders are indeed solutions to the robust DRO statistic. 

As an example, let us fix $\varepsilon < 2 \min_{\sigma \in \frak{S}_n} p(\sigma)$, let us write $\sigma^* = \sigma^{med}_{p,d_{\tau}}$ the Kemeny median for Kendall-tau distance and let us fix $\sigma \in \frak{S}_n$ and $\tau$ a transposition. Then, let's define the following distribution set

\begin{equation*}
    \begin{split}
    \mathcal{U}_{\varepsilon, \sigma, \tau} = \left\{ p \in \Delta^{n!} \; | \; : \forall \nu \neq \sigma, \sigma\tau, \, p(\nu)=\frac{1-\eta}{n!} \right. \\
     p(\sigma\tau) \in [\max(\frac{1-\eta}{n!}, p(\sigma) - \varepsilon)], \\
     \left. p(\sigma) \in [\frac{1-\eta}{n!}, 1], \, \forall \eta \in [0, 1-n! \varepsilon] \right\}
    \end{split}
\end{equation*}

On the set $\mathcal{U}_{\varepsilon, \sigma, \tau}$, which is of positive mass, the DRO statistic is a non-strict bucket order. 

Here is a sketch of proof. Define $p \in \mathcal{U}_{\varepsilon, \sigma, \tau}$ the following distribution: $\forall \nu \neq \sigma, \sigma \tau, \,  p(\nu) = \frac{1-\eta}{n!}; p(\sigma) = \frac{1-\eta}{n!} + \eta - \lambda$ and $p(\sigma \tau) = \frac{1-\eta}{n!} + \lambda$ for a $\eta \in [0, 1-n! \varepsilon], \; \lambda \in [\max(0, \frac{\eta - \varepsilon}{2}), \frac{\eta}{2}]$.

It can be easily checked that $\sigma = \sigma^{med}_{p, d_{\tau}}$. Moreover, the adversarial distribution for the DRO (i.e. the inner max part) is the following: $\forall \mu \neq \nu, \nu_{opp} \; q_{\varepsilon, \nu}(\mu)= p(\mu), \, q_{\nu}(\nu) = p(\nu) - \varepsilon/2$ and $q_{\nu}(\nu_{opp}) = p(\nu) + \varepsilon/2$. Then, let's write $\pi = \{\sigma, \sigma \tau\}$ we have the following result: $q_{\sigma}^T D_{\tau} \sigma - q_{\pi}^T D_{\tau} \pi = q_{\sigma}^T D_{\tau} \sigma - q_{\sigma}^T D_{\tau} \pi = \frac{1}{2}(p(\sigma \tau) - p(\sigma) + \varepsilon) \geq 0$.

\newpage
\section{Alternative Formulation for Algo}

Let $\pi\in\wO$ be  a bucket ranking and remember that $\pi^{(i)}$ denotes the $i^{\rm th}$ bucket of $\pi$. Let $P$ be a pairwise marginal matrix $P$, we define

$\bar{P}_{ij}(\pi) = \max \left\{\left|P_{l,l'} - \frac{1}{2}\right| : (l,l')\in\pi^{(m)}\times\pi^{(m')}, (m,m')\in[n]^2 ~s.t.~ i\leq m \leq m'\leq j\right\}$

$\cG(\pi,t) = \left\{(i,j)\in [n]^2: \bar{P}_{ij}(\pi) \leq t\right\}$

\begin{algorithm}
\DontPrintSemicolon
\SetKwInOut{Input}{Input}
\SetKwInOut{Output}{Output}
\Input{Pairwise matrix $P$, Ranking median $\sigma$, threshold $t \in [0, 0.5]$.}
$\pi \gets \sigma$ \tcp*{$\sigma$ being a specific bucket order}
\While{$\cG(\pi, t) \neq \emptyset$}{
    $(i^*, j^*) = \argmin_{(i,j)\in\cG(\pi,t)} \bar{P}_{ij}(\pi)$ \;
    update $\pi$ by merging all buckets between $i^*$ and $j^*$
    \vskip -2em
    \begin{flushleft}
        \begin{flalign*} 
            \begin{cases}
                \pi^{(i)} &\gets \pi^{(i)} ~~~\text{for}~ i < i^*\\
                \pi^{(i^*)} & \gets \bigcup_{l\in[n], i^*\leq l\leq j^*}\pi^{(l)}\\
                \pi^{(i - j^* + i^*)} & \gets \pi^{(i)} ~~~\text{for}~ i > j^*
            \end{cases}&&
        \end{flalign*}
    \end{flushleft}
    }
    \Output{$\pi$}
\caption{Na\"ive Merge}
\label{algo_maxpair}
\end{algorithm}

\begin{algorithm}
\DontPrintSemicolon
\SetKwInOut{Input}{Input}
\SetKwInOut{Output}{Output}
\Input{Pairwise matrix $P$, Ranking median $\sigma$, threshold $t \in [0, 0.5]$.}
$\pi \gets \sigma$ \tcp*{$\sigma$ being a specific bucket order}
\While{$\cG(\pi, t) \neq \emptyset$}{
    $(i^*, j^*) = \argmax_{(i,j)\in\cG(\pi,t)} \bar{P}_{ij}(\pi)$ \;
    update $\pi$ by merging all buckets between $i^*$ and $j^*$
    \vskip -2em
    \begin{flushleft}
        \begin{flalign*} 
            \begin{cases}
                \pi^{(i)} &\gets \pi^{(i)} ~~~\text{for}~ i < i^*\\
                \pi^{(i^*)} & \gets \bigcup_{l\in[n], i^*\leq l\leq j^*}\pi^{(l)}\\
                \pi^{(i - j^* + i^*)} & \gets \pi^{(i)} ~~~\text{for}~ i > j^*
            \end{cases}&&
        \end{flalign*}
    \end{flushleft}
    }
    \Output{$\pi$}
\caption{Downward Merge}
\label{algo_maxpair}
\end{algorithm}

\section{Material removed}

Moreover, inter-buckets ranking remains challenging in a general case, which can be addressed when restricting the analysis to \textit{(Strictly) Stochastically Transitive} distributions.

\begin{definition}
    {\sc (Stochastic transitivity)} A distribution $p\in\cM_+^1(\pS)$ is said to be stochastically transitive (ST) iif $\forall \, (i,j,k) \in [\![1,n]\!], P_{i,j} \geq 1/2$ and $P{j,k} \geq 1/2 \Rightarrow P_{i,k} \geq 1/2$. It is said to be strictly stochastically transitive if the inequalities are strict.
\end{definition}

When distribution $p\in\cM_+^1(\pS)$ is SST, the pairwise matrices provide a simpler way to characterize Kemeny's median:

\begin{remark} {\sc (Uniqueness of the ranking median)} Let $p \in \Delta^{\frak{S}_n}$ be a SST distribution, and let $d_{\tau}$ be Kendall-tau distance. Then, the median $\sigma^{med}_{d_{\tau}}(p)$ is unique and can be defined as $\forall i \in [\![1, n ]\!],  \sigma^{med}_{d_{\tau}}(p)(i) = 1 + \sum_{k \neq i} \mathbb{1}(P_{i,k} < 1/2)$~ \cite{Korba2017}.
\label{rk:sst_unique}
\end{remark}

This result derives from the definition of SST distributions and the following simplification remark.

\begin{remark} {\sc Pairwise matrix simplification.} Let $d_{\tau}$ be the Kendall-tau distance, $p\in\cM_+^1(\pS)$ a distribution and $\sigma \in \frak{S}_n$ a ranking. Then $\mathbb{E}_{\Sigma \sim p}(d_{\tau}(\Sigma, \sigma)) = \sum_{i<j} P_{i,j} \mathbb{1}(\sigma(i) > \sigma(j)) + (1-P_{i,j})\mathbb{1}(\sigma(i) < \sigma(j))$~ \cite{Korba2017}.
\label{rk:pairwise_simpl}
\end{remark}

\begin{algorithm}
\SetKwInOut{Input}{Input}
\SetKwInOut{Output}{Output}
\Input{Pairwise matrix $P$ of a SST distribution, threshold $t \in [0, 0.5]$.}
\Output{Naïve Merge statistic $\pi^{merge}(p)$}
\While{$\exists (i,j)$ s.t. $i<j, |P_{i,j} - 1/2| \leq t$}{
    $(i^*, j^*) = \argmin_{i<j} |P_{i,j} - 1/2|$ \;
    Put $(i^*, j^*)$ in the same bucket \;
    Update pairwise matrix $P$: $\forall i,j, \; P_{i^*, j} = P_{j^*,j} = max(P_{i^*,j} , P_{j^*,j}); \; P_{i,i^*} = P_{i, j^*} = max(P_{i,i^*}, P_{i,j^*})$ and $P_{i^*,j^*} = 1/2$
    }
    Return $\pi^{NM}(p)$ s.t. $\forall i \in [\![1,n]\!]\, \pi^{NM}(p)(i) = 1 + \sum_{k \neq i} \mathbb{1}(P_{i,k} < 1/2)$
\caption{Naïve Merge Algorithm}
\label{algo_merge}
\end{algorithm}

\begin{algorithm}
\SetKwInOut{Input}{Input}
\SetKwInOut{Output}{Output}
\Input{Pairwise matrix $P$ of a SST distribution, threshold $t \in [0, 0.5]$.}
\Output{Downward Merge statistic $\pi^{maxpair}(p)$}
\While{$\exists (i,j)$ s.t. $|P_{i,j} - 1/2| \leq t$}{
    $(i^*, j^*) = \argmin_{i,j : i \succ j} \left| |P_{i,j} - 1/2|- t \right|$ \;
    $\forall \, l \text{ s.t. } i^* \succ l \succ j^*$ and s.t. $|P_{i^*,l} - 1/2| \leq t$ and $|P_{l,j^*}-1/2| \leq t$ put $i^*, j^*, l$ in the same bucket \;
    Update pairwise matrix $P$: $\forall i,j, \; P_{i^*, j} = P_{j^*,j} = P_{l,j} = \max(P_{i^*, j}, P_{j^*,j}, \{P_{l,j}\}); \; P_{i,i^*} = P_{i, j^*} = P_{i,l} = \max(P_{i,i^*}, P_{i, j^*}, \{P_{i,l}\})$ and $P_{i^*,j^*} = P_{i^*,l} = P_{l,j^*} = 1/2$
    }
    Return $\pi^{DM}(p)$ s.t. $\forall i \in [\![1,n]\!]\, \pi^{DM}(p)(i) = 1 + \sum_{k \neq i} \mathbb{1}(P_{i,k} < 1/2)$
\caption{Downward Merge Algorithm}
\label{algo_maxpair}
\end{algorithm}
