# Supplementary material for: Robust Consensus in Ranking Data Analysis: Definitions, Properties and Computational Issues
Source: arXiv:2303.12878 source file (2023-03-22)
Supplement: Supplementary file 2 [file X_appendix_dro.tex]

\section{Bucket Orders are Optimal for the DRO Statistics}
\label{app:dro}

\begin{restatable}{proposition}{propbucketorderoptimalfordro}\label{prop:bucket_order_optimal_for_dro}
$\exists p \in \cM_+^1(\pS), \sigma\in\pS, r\in[n-1]$ s.t. 
\begin{align*}
    \{\sigma, \tau_{r,r+1}\sigma\} = \argmin_{S \subseteq \pS} \max_{q: \textsc{tv}(p,q)\leq \varepsilon} \lE_{\Sigma\sim q}\left[\max_{\sigma\in S}d(\Sigma, \sigma)\right]
\end{align*}
\end{restatable}

\begin{proof}
    For $\eta, \lambda\in[0,1]$, let $\sigma_0\in\pS$, $r\in[n-1]$ and $p\in\distribs$ be such that for any $\sigma\in\pS$,
    \begin{align}
    p(\sigma) =
        \begin{cases}
        \frac{1-\eta}{n!} + \lambda & \text{if }\nu =\tau_{r,r+1} \sigma_0\\
        \frac{1-\eta}{n!} + \eta - \lambda & \text{if }\nu = \sigma_0\\
        \frac{1-\eta}{n!} & \text{otherwise.}
        \end{cases}
    \end{align}

    Given $S\subseteq\pS$, we denote $q_S = \argmax_{q: \textsc{tv}(p,q)\leq \varepsilon}\lE_{\Sigma\sim q}\left[\max_{\sigma\in S}d(\Sigma, \sigma)\right]$. 
\end{proof}
